# Supplementary material for: Interpretable Explanations of Black Boxes by Meaningful Perturbation
Source: arXiv:1704.03296 source file (2021-12-03)
Supplement: Supplementary file 1 [file supplementary.tex]

\section{Supplementary Materials}
%\begin{figure}[t]
%\begin{center}
%  \includegraphics[width=0.9\linewidth]{animal_parts_sorted_diff.pdf}
%\end{center}
%   \caption{Animal Parts Experiment}
%\label{fig:animal_parts}
%\end{figure}
